# Supplementary material for: Microscopic origins of the anomalous melting behaviour of high-pressure sodium
Source: arXiv:1110.2031 source file (2011-10-10)
Supplement: Supplementary file 1 [file Supplmentary.pdf]

# Supplementary Information for "Microscopic origins of the anomalous melting behaviour of high-pressure sodium"

Hagai Eshet, Rustam Z. Khaliullin, Thomas D. Kühne,
Jörg Behler, Michele Parrinello

September 21, 2011

*Structural and electronic transitions in liquid sodium.* The only hypothesis that has been proposed to explain physical origins of anomalous melting attributes this behaviour to a series of pressure induced structural and electronic transitions in the liquid [1]. According to *ab initio* molecular dynamics (MD) simulations of Raty *et al.* [1], liquid sodium undergoes a progressive transition from the bcc- to fcc-like local order around 30 GPa. It has also been suggested that an opening of the pseudogap in the electronic density of states above ∼60 GPa drives yet another transition, in which the liquid acquires the cI16-like local structure [1]. While these conclusions are highly appealing first-principle MD simulations performed by Hernández *et al.* [3] show no evidence of structural transitions in liquid in the region of the anomalous melting behaviour. Yamane *et al.* [2] have attributed the discrepancy between these results to a different treatment of the semicore states, which were explicitly included in one case [3] and incorporated into the pseudopotential in the other [1]. They have shown that the semicore states play an important role in determining the structure of liquid at high pressures [2].

To verify the existence of structural and electronic transitions in the liquid phase we evaluated the order parameter introduced in Ref. [1] for liquid sodium in the 0–140 GPa range along the calculated melting curve. Our calculations do not reveal any significant changes in the structural properties of high-density liquid sodium (Supplementary Fig. 5A). In addition,

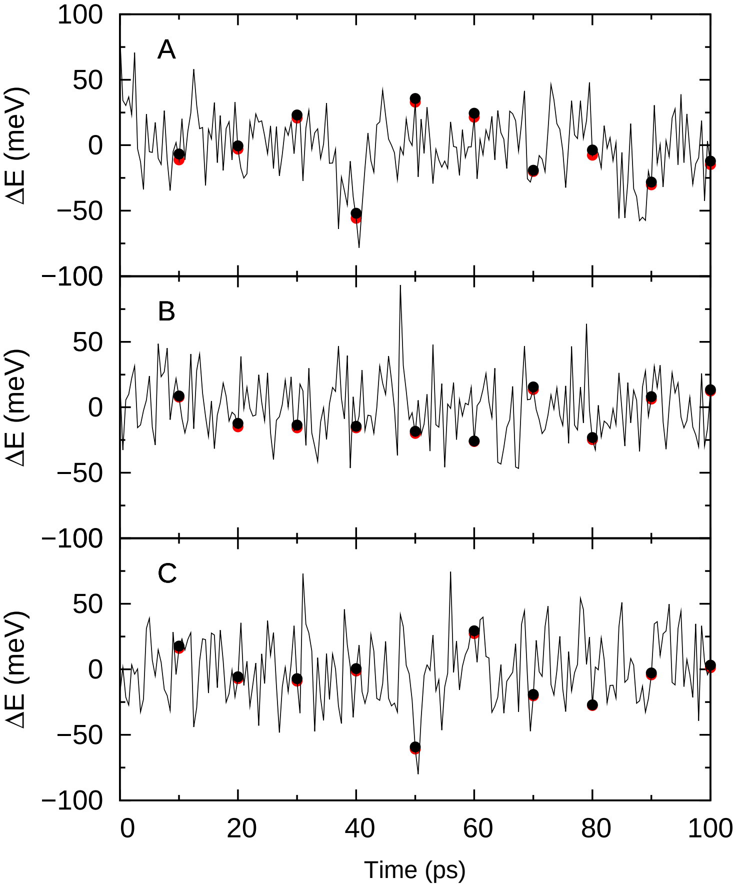


Figure 1: Comparison of the energies obtained with the NN potential (red dots) and PBE density functional (black dots) for structures encountered in MD simulation of liquid sodium in the relevant P–T range. The black line shows the magnitude of the energy fluctuations in the simulations. a. 90 GPa, 1100 K. b. 60 GPa, 1200 K. c. 30 GPa, 1200K.

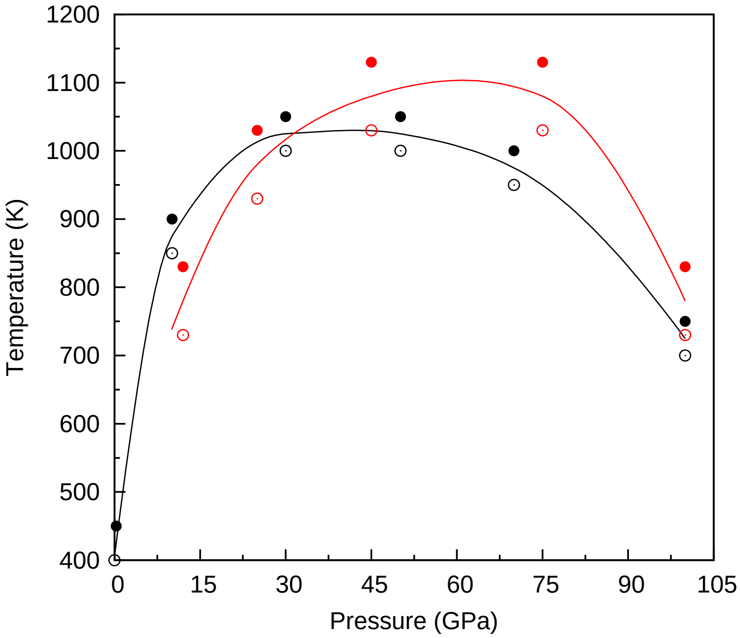


Figure 2: The "heat-until-it-melts" curves obtained with *ab initio* simulations [2] (red) and the NN potential (black). For comparison purpose small simulation cells were used. Points below 90 GPa were obtained by melting the bcc phase (54 atoms in the cell), points above 90 GPa by melting the fcc phase (128 atoms).

Table 1: Density-dependent fitting parameters used to reproduce DFT jellium potential with the analytical equation below[a].

| $\rho_e$, $\mathring{A}^{-3}$ | $A$, kJ mol$^{-1}$ | $B$, kJ mol$^{-1}$ $\mathring{A}^m$ | $r_0$, $\mathring{A}$ | $k_0$, $\mathring{A}^{-1}$ | $k_F$ [b], $\mathring{A}^{-1}$ | $m$ |
|---|---|---|---|---|---|---|
| 0.025 | 907521 | 5643.12 | 0.668038 | 4.70328 | 0.905 | 5.28656 |
| 0.040 | 534313 | 6562.03 | 1.018580 | 4.04097 | 1.058 | 5.58567 |
| 0.060 | 387396 | 6770.53 | 1.230760 | 3.70687 | 1.212 | 5.79208 |
| 0.080 | 222572 | 5160.46 | 1.311630 | 3.38107 | 1.334 | 5.67845 |
| 0.090 | 215154 | 4878.10 | 1.329670 | 3.36481 | 1.387 | 5.65150 |

[a] $\phi(r) = Ar^{-1}\exp(-k_0 r) + Br^{-m}\cos[2k_F(r - r_0)]$.

[b] Fermi wavenumber is calculated as $k_F = \sqrt[3]{3\pi^2\rho}$ (i.e. it is not a fitting parameter).

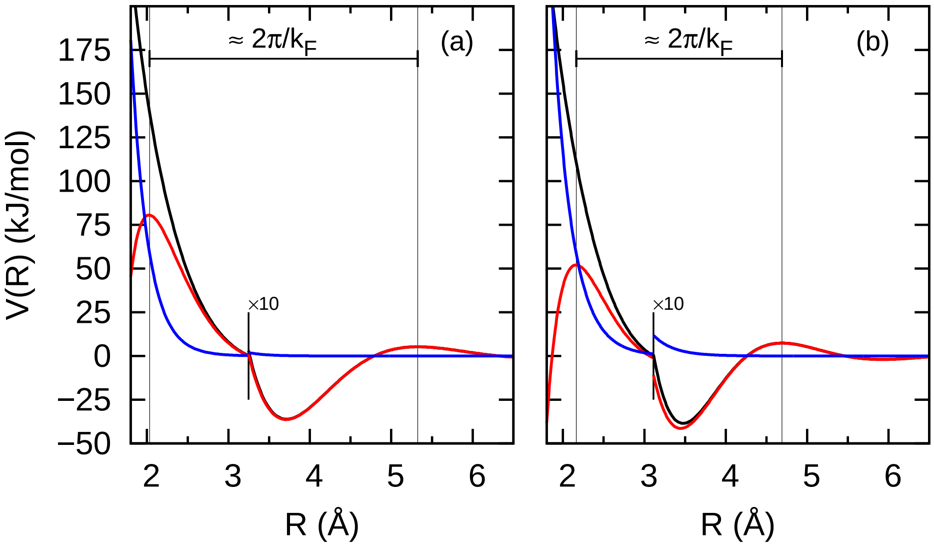


Figure 3: Decomposition of the sodium pair potential (black) into the repulsive Yukawa potential (blue) and oscillatory term (red). The period of oscillations is determined by the density-dependent Fermi wavenumber $k_F$: a. 10 GPa, b. 90 GPa.

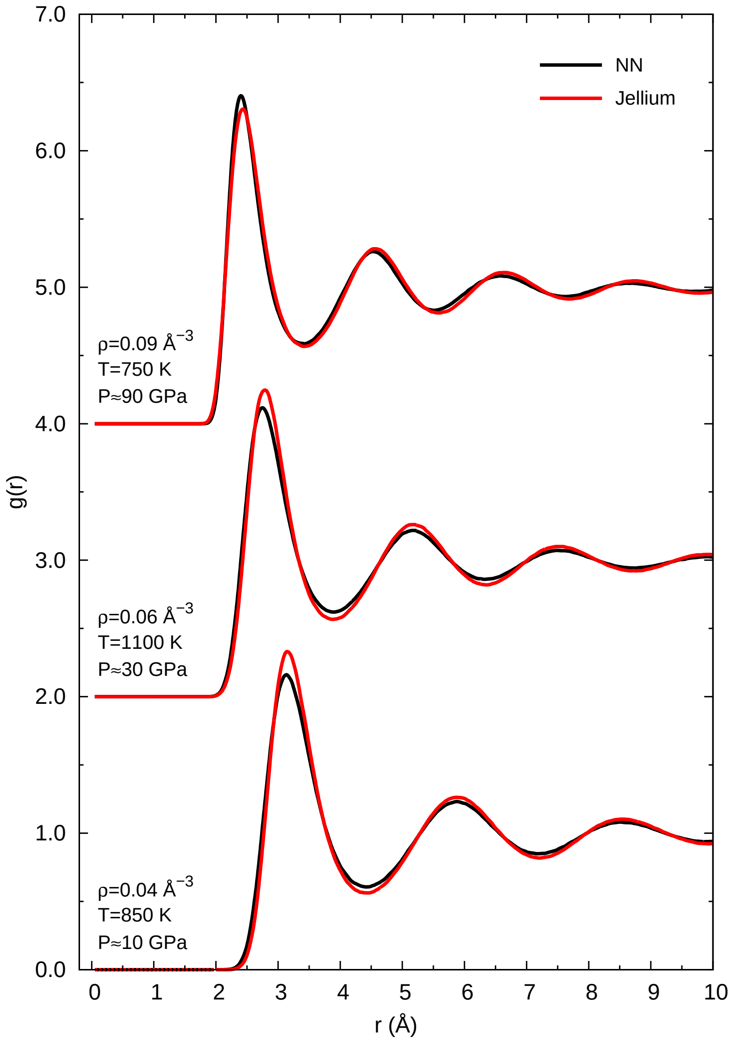


Figure 4: RDFs obtained from simulations with the NN potential (black) and the jellium pair potential (red).

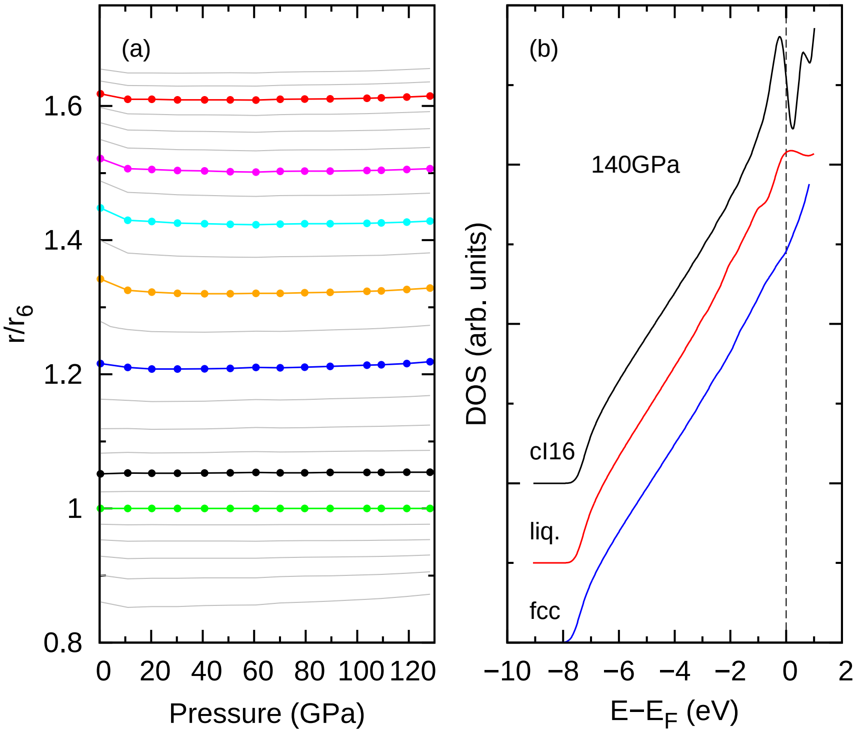


Figure 5: a. Pressure dependence of the average interatomic distances to the first, second, etc. nearest neighbours along the melting curve in liquid sodium. Distances are normalized to the sixth-nearest neighbour (compare to Fig. 2a in Ref. [1]). b. Electronic density of states in fcc (350 K), cI16 (0 K) and liquid (450 K) sodium at 140 GPa calculated with PBE for structures obtained from NN-driven MD simulations (compare to Fig. 3b in Ref. [1]).

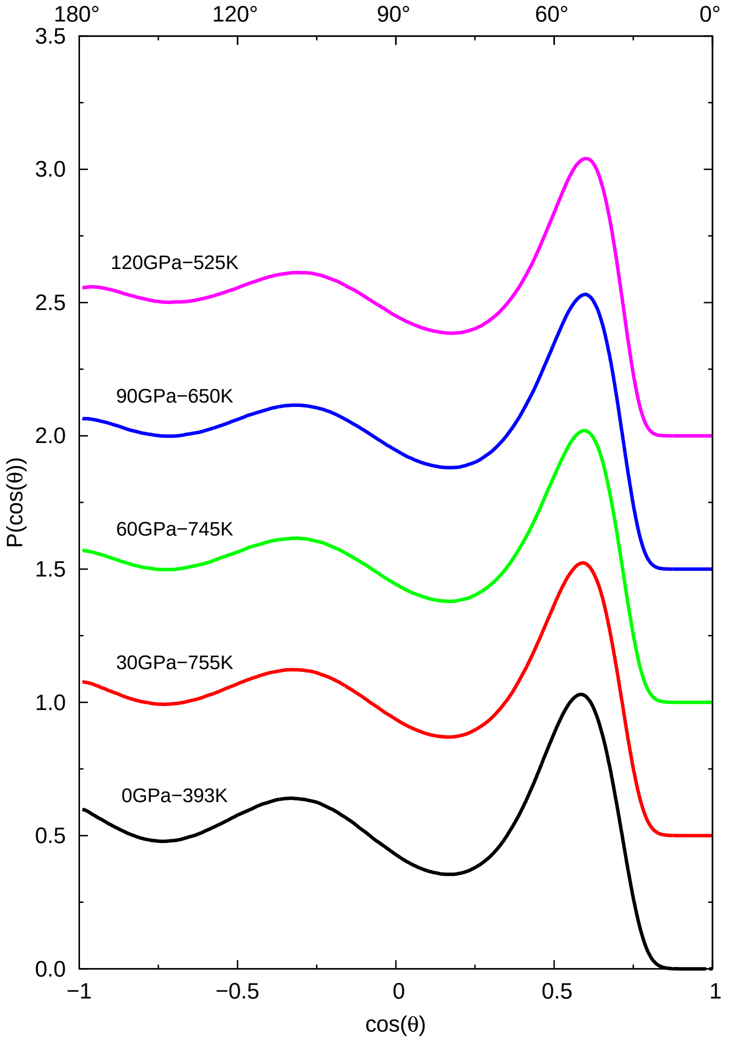


Figure 6: Angular bond distribution obtained for liquid states along the melting curve from NN-driven simulations.

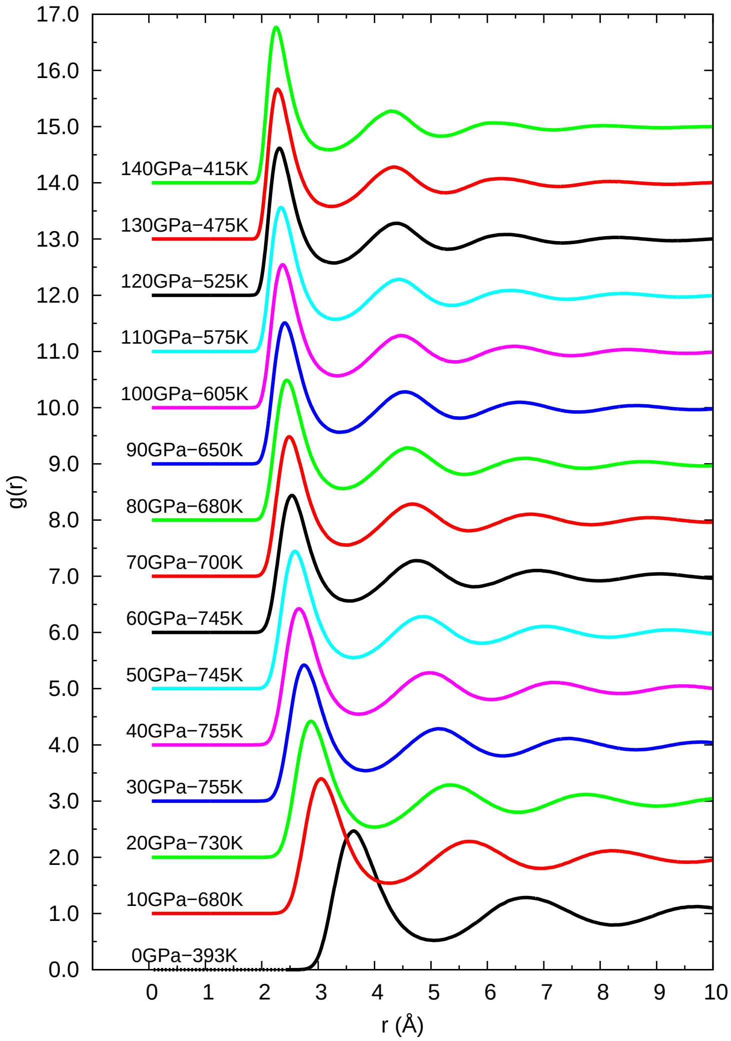


Figure 7: RDFs obtained for liquid states along the melting curve from NN-driven simulations (compare to Supplementary Fig. S2 in Ref. [1]).

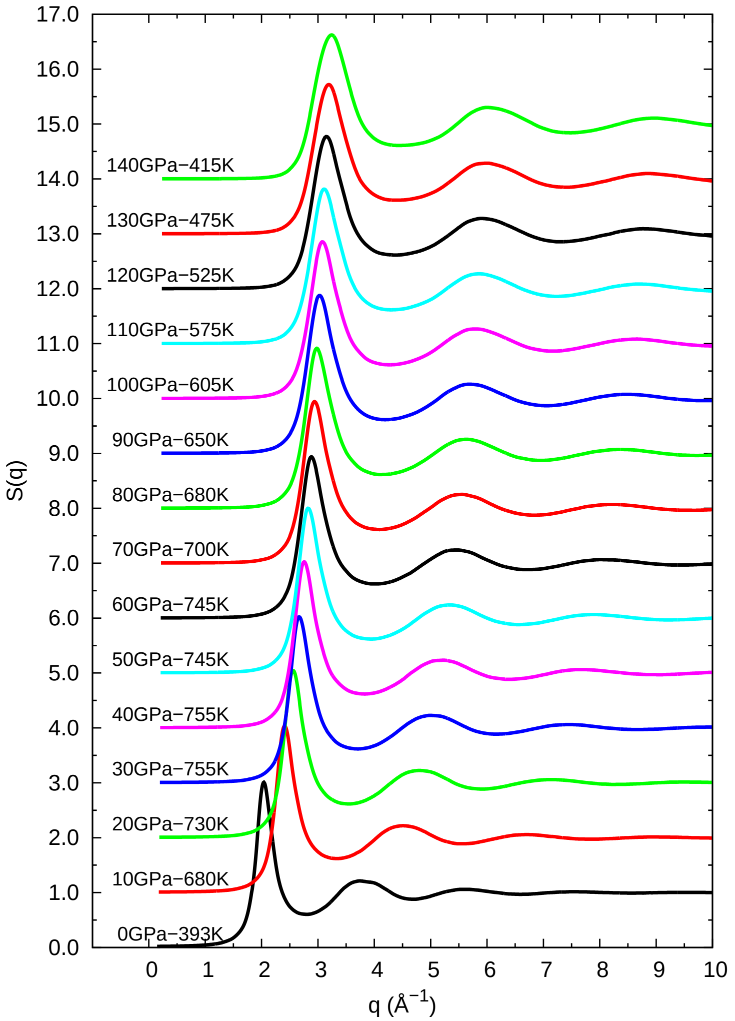


Figure 8: Structure factors obtained for liquid states along the melting curve from NN-driven simulations.(compare to Supplementary Fig. S1 in Ref. [1]).

the electronic density of states calculated with DFT for liquid structures collected from NN-driven MD simulations above the cI16 phase does not show a pseudogap, which is clearly visible in the solid phase (Supplementary Fig. 5B). Analysis of the pressure dependence of other structural properties does not show noticeable structural changes in the 0–140 GPa range (Supplementary Fig. 6-8). Discrepancies between our results and Ref. [1] can be attributed in part to the different treatment of the $2s$ and $2p$ semicore electrons [2] and also to the larger system size and the longer simulation times performed in this work.

*Pressure decomposition analysis.* To understand why liquid sodium becomes denser than the solid bcc and fcc phases, we calculated and compared the pressure for the solid and liquid phases at melting temperatures ($T_m$) and fixed densities ($\rho$) in three regions of the phase diagram: ~0 GPa (normal melting behaviour), ~35 GPa (slightly above the maximum of the melting curve) and ~100 GPa (anomalous behaviour). The difference in pressure between the liquid and solid phases $\Delta P(\rho) \equiv P_s(\rho) - P_l(\rho)$ is negative at low densities (i.e. the solid is denser than the liquid) but changes the sign at the densities corresponding to ~30 GPa.

The macroscopic pressure can be expressed in terms of the radial distribution function $g(r)$:

$$P(\rho) = \rho k_B T - \frac{2\pi}{3}\rho^2 \int_0^r \frac{d\phi(r)}{dr} g(r) r^3 dr. \tag{1}$$

The pairwise nature of the effective jellium potential allowed us to analyse contributions of different regions of the potential $\phi(r)$ to the total $\Delta P(\rho)$. The contribution of atoms located within a sphere of radius $r$ from a central atom is defined as

$$\Delta P(r, \rho) = -\frac{2\pi}{3}\rho^2 \int_0^r \frac{d\phi(r)}{dr} \left[g_s(r) - g_l(r)\right] r^3 dr, \tag{2}$$

where $g_s(r)$ and $g_l(r)$ are the radial distribution functions for the solid and liquid phases at $T_m$, respectively.

As expected, $\Delta P(r, \rho)$ converges to the negative value as $r \to \infty$ in the region of the normal melting behaviour and to the positive value in the region of the anomalous slope (Supplementary Fig. 9). It can be seen from Supplementary Fig. 9 that the converged value of $\Delta P(r, \rho)$ is determined largely by the short-range behaviour of potential (i.e. by the region of the repulsive wall where the gradient is large).

As evident from the decomposition of the effective potential (Eq. 1 in the main text) the soft region in the repulsive wall is induced by a maximum of the oscillatory term (Supplementary Fig. 3). The position of the maximum shifts towards higher distances as pressure

increases and, above certain pressure, the soft region starts affecting the interactions between closest atoms. This makes the initial dip in $\Delta P(r,\rho)$ shallower and pushes $\Delta P(\infty,\rho)$ to positive values, hence resulting in the drop of the melting temperatures.

The long-range behaviour of $\Delta P(r,\rho)$ at 35 GPa shows (Supplementary Fig. 9) that the long-range oscillations also contribute to the anomalous melting. However, while being essential for determining the precise position of the melting line the long-range oscillatory component is less important for the overall reentrant effect (see Fig. 2 in the main text).

# References

[1] Raty, J. Y.; Schwegler, E.; Bonev, S. A. *Nature* **2007**, *449*, 448.

[2] Yamane, A.; Shimojo, F.; Hoshino, K. *J. Phys. Soc. Jpn.* **2008**, *77*(6), 064603.

[3] Hernandez, E. R.; Iniguez, J. *Phys. Rev. Lett.* **2007**, *98*(5), 055501.

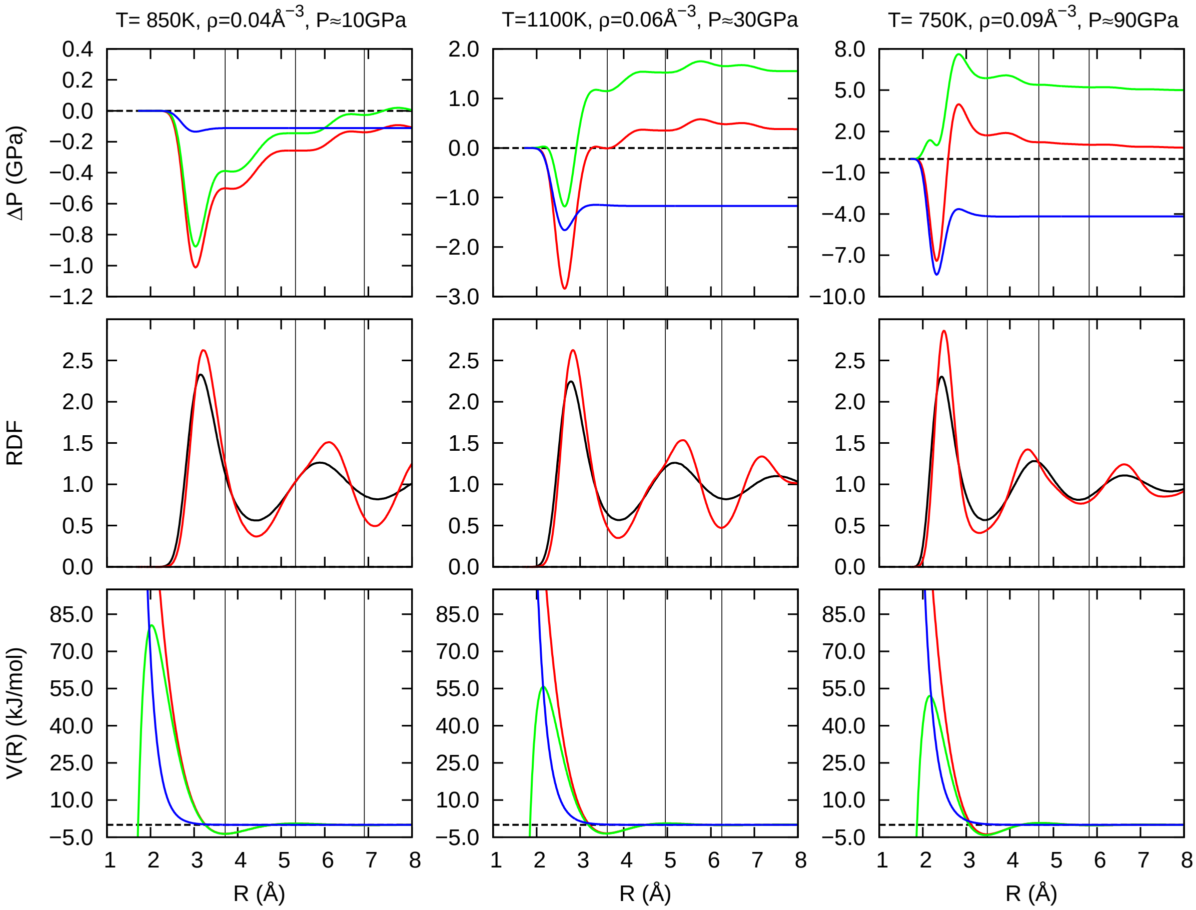


Figure 9: Pressure decomposition analysis. Lower panels: effective pair potential (red) obtained from the jellium model and its decomposition into the Yukawa (blue) and oscillatory (green) terms. Middle panel: RDFs of liquid (black) and solid (red) phases. Upper panel: pressure curve given by Eq. 2 (red) and the corresponding Yukawa (blue) and oscillatory (green) components.
